# Supplementary material for: Uniform Convergence of Gradients for Non-Convex Learning and Optimization
Source: arXiv:1810.11059 source file (2018-11-11)
Supplement: Supplementary file 1 [file appendix_scratch.tex]

% !TEX root = paper.tex

\section{Scratch---to be removed}
\subsection{Notation}
\begin{itemize}
\item Instances $\cX$, labels/outcomes $\cY$, function class $\cF:\cX\to\cY$ or $\cG:\cX\to\cY$, $\cZ $ is $\cX \times \cY$
\item Weight/parametric model set: $\cW\subset{}\bbR^{d}$. Parametric function class $f_{w}:\cX\to\cY$, $w\in\cW$.
\item Loss $\ls(w\midsem{}x_t, y_t)$ or $\ls_{t}(w)$.
\item Data distribution $(x,y)\sim{}\cD$. $\En_{(x,y)\sim\cD}$ or $\En_{\cD}$ for short. $L_{\cD}$: in-expectation version of loss above.
  \item $\wh{L}_{n}$ --- empirical loss.
  \item $\nabla \ls(w\midsem{}x_t, y_t)$ is the gradient, $\nabla^2 \ls(w\midsem{}x_t, y_t)$ is the hessian, similarly $\nabla \emprisk(w)$, $\nabla^2 \emprisk(w)$, $\nabla \poprisk(w)$, $\nabla^2 \poprisk(w)$
\item Norm $\nrm*{\cdot}$, dual norm $\nrm*{\cdot}_{\star}$
\item For vector valued function classes $\cF\subseteq{}\cX\to\bbR^{K}$, $K$ is the default notation for output dimension.
\ascomment{Should change this, K suits better for the number of clusters}\dfcomment{they coincide here, so i'm fine with keeping same}
\item For neural nets, $d_0$ is dimension of input, $d_1$ dimension of first hidden layer, ...
\item Neural nets: Parameters are $W_{1}$,\ldots,$W_{L}$. Activations are $\sigma$.
\item $\trn$ denotes transpose, $\tens$ denotes kronecker product (not outer product).
\item $\eps$: scalar rademacher, $\mb{\eps}$: vector rademacher
\item Margin parameters: $\gamma$, $\phi$.
  \item Algorithm names use texstsf font (eg \glmtron)
\item Unit ball $\bbB^{d}_{2}(r)$ etc.
\item Derivatives: See preliminaries, plus directional derivatives in the appendix. No directional derivatives in the main body.
\item $B$: Bound on parameter norm.
\item $R$: Bound on $x_t$ norm.
\item $G$: bound on $\nrm*{\grad{}\ls}$.
\item Dataset size $n$.
\end{itemize}

\subsection{Related work}
\dfcomment{delete}
\textbf{Recent generalization theory}
\cite{bartlett2017spectrally, neyshabur2017exploring, neyshabur2017pac, arora2018stronger, golowich2017size}

maybe: \cite{zhou2018compressibility}

\textbf{Recent experimental works}
\dfcomment{Tempted to ignore these; this is not a pure neural net paper.}

\cite{zhang2016understanding, keskar2016large}

maybe:
  \cite{dziugaite2017computing, novak2018sensitivity, dinh2017sharp}
